# Supplementary material for: Revisiting Realistic Test-Time Training: Sequential Inference and Adaptation by Anchored Clustering Regularized Self-Training
Source: arXiv:2303.10856 source file (2023-03-20)
Supplement: Supplementary file 1 [file Appendix.tex]

\subsection{Detailed Results}

We provide details of test-time training on CIFAR10-C, CIFAR100-C and ModelNet40-C datasets in Tab.~\ref{tab:cifar10c},~\ref{tab:cifar100c} and ~\ref{tab:modelnet40c} respectively. The results in Tab.~\ref{tab:cifar10c} and ~\ref{tab:cifar100c} suggest TTAC has a powerful ability to adapt to the corrupted images, and obtains the state-of-the-art performances on almost all corruption categories. 

\begin{table*}[!htb]
    \centering
    \caption{The results of CIFAR10-C under the sTTT protocol}
    \resizebox{\linewidth}{!}{
        \begin{tabular}{l|ccccccccccccccc|c}
        \toprule
        Method & Brit & Contr & Defoc & Elast & Fog & Frost & Gauss & Glass & Impul & Jpeg & Motn & Pixel & Shot & Snow & Zoom & Avg \\
        \midrule
        TEST & 7.00 & 13.28 & 11.84 & 23.38 & 29.42 & 28.25 & 48.73 & 50.79 & 57.01 & 19.46 & 23.38 & 47.88 & 44.00 & 21.93 & 10.84 & 29.15 \\
        BN   & 8.21 & 8.36  & 9.73  & 19.43 & 20.16 & 13.72 & 17.46 & 26.34 & 28.11 & 14.00 & 13.90 & 12.22 & 16.64 & 16.00 & 8.03  & 15.49 \\
        TENT & 8.22 & 8.07  & 9.93  & 18.29 & 15.65 & 14.14 & 16.60 & 24.10 & 25.80 & 13.39 & 12.34 & 11.06 & 14.75 & 13.87 & 7.87  & 14.27 \\
        T3A  & 8.33 & 8.70 & 9.70 & 19.51 & 20.26 & 13.83 & 17.27 & 25.61 & 27.63 & 14.05 & 14.26 & 12.12 & 16.37 & 15.78 & 8.13 & 15.44 \\
        SHOT & 7.58 & 7.78  & 9.12  & 17.76 & 16.90 & 12.56 & 15.99 & 23.30 & 24.99 & 13.19 & 12.59 & 11.37 & 14.85 & 13.75 & 7.51  & 13.95 \\
        TTT++ & 7.70 & 7.91 & 9.24 & 17.55 & 16.39 & 12.74 & 15.49 & 22.57 & 22.86 & 13.02 & 12.52 & 11.46 & 14.45 & 13.90 & 7.51 & 13.69 \\
        TTAC & 6.41 & 8.05 & 7.85 & 14.81 & 10.28 & 10.51 & 13.06 & 18.36 & 17.35 & 10.80 & 8.97 & 9.34 & 11.61 & 10.01 & 6.68 & 10.94 \\
        TTAC+SHOT & 6.37 & 6.98 & 7.79 & 14.80 & 11.04 & 10.52 & 13.58 & 18.34 & 17.68 & 10.94 & 8.93 & 9.20 & 11.81 & 10.01 & 6.79 & 10.99 \\
        TTAC++ & \textbf{5.59} & \textbf{6.28} & \textbf{7.53} & \textbf{12.99} & \textbf{8.95} & \textbf{9.22} & \textbf{12.13} & \textbf{15.79} & \textbf{14.37} & \textbf{10.65} & \textbf{8.70} & \textbf{8.60} & \textbf{10.70} & \textbf{8.82} & \textbf{6.37} & \textbf{9.78} \\
        \bottomrule
        \end{tabular}
    }
    \label{tab:cifar10c}
\end{table*}

\begin{table*}[!htb]
    \centering
    \caption{The results of CIFAR100-C under the sTTT protocol}
    \resizebox{\linewidth}{!}{
        \begin{tabular}{l|ccccccccccccccc|c}
        \toprule
        Method & Brit & Contr & Defoc & Elast & Fog & Frost & Gauss & Glass & Impul & Jpeg & Motn & Pixel & Shot & Snow & Zoom & Avg \\
        \midrule
        TEST & 28.84 & 50.87 & 39.61 & 59.53 & 68.10 & 60.21 & 80.77 & 82.27 & 87.75 & 49.98 & 54.20 & 72.27 & 77.84 & 54.57 & 38.36 & 60.34 \\
        BN   & 31.78 & 33.06 & 33.86 & 48.65 & 54.23 & 42.28 & 48.02 & 57.08 & 60.14 & 39.09 & 40.72 & 37.76 & 45.83 & 46.31 & 31.91 & 43.38 \\
        TENT & 30.45 & 31.47 & 32.48 & 45.84 & 44.85 & 41.39 & 45.59 & 52.31 & 56.16 & 38.94 & 38.41 & 35.55 & 43.40 & 42.89 & 31.10 & 40.72 \\
        T3A   & 31.66 & 32.63 & 33.62 & 47.60 & 53.06 & 41.95 & 46.63 & 55.51 & 58.92 & 38.89 & 40.26 & 37.21 & 45.32 & 46.08 & 31.43 & 42.72 \\
        SHOT & 29.36 & 30.49 & 31.33 & 43.41 & 45.14 & 39.31 & 43.35 & 50.98 & 53.75 & 36.07 & 36.11 & 34.54 & 42.16 & 40.99 & 29.52 & 39.10 \\
        TTT++ & 30.79 & 31.48 & 33.04 & 44.95 & 47.74 & 40.19 & 43.94 & 52.06 & 54.08 & 37.26 & 38.10 & 35.40 & 42.28 & 42.97 & 30.58 & 40.32 \\
        TTAC & 28.13 & 32.55 & 29.45 & 41.54 & 39.07 & 36.95 & 40.01 & 48.30  & 49.21 & 34.55 & 33.29 & 32.69 & 38.62 & 37.69 & 27.61 & 36.64 \\
        TTAC+SHOT & 27.73 & 32.19 & \textbf{29.25} & 41.26 & 38.67 & 36.67 & 40.01 & 47.87 & 49.21 & \textbf{34.13} & 32.98 & 32.52 & 38.62 & 37.35 & \textbf{27.36} & 36.39 \\
        TTAC++ & \textbf{26.20} & \textbf{26.47} & 29.84 & \textbf{41.11} & \textbf{37.65} & \textbf{36.13} & \textbf{39.24} & \textbf{47.51} & \textbf{48.52} & 34.78 & \textbf{32.26} & \textbf{31.18} & \textbf{38.06} & \textbf{35.59} & 27.72 & \textbf{35.48} \\
        \bottomrule
        \end{tabular}
    }
    \label{tab:cifar100c}
\end{table*}
